# Supplementary material for: Compositional Diffusion-Based Continuous Constraint Solvers
Source: arXiv:2309.00966 source file (2023-09-02)
Supplement: Supplementary file 1 [file 2-supplementary.tex]

\documentclass{article}

\usepackage{corl_2023} %

\usepackage{booktabs}
\usepackage{multirow}

\input{inc-math}
\input{inc-packages}
\input{inc-macros}

\title{Supplementary Materials to \\ Compositional Diffusion Constraint Solvers}

\author{
  Zhutian Yang, \, Yilun Du, \,Leslie P. Kaelbing, \,Tomás Lozano-Pérez, \,Jiayuan Mao\\
  Department of Electrical Engineering and Computer Sciences\\
  Massachusetts Institute of Technology 
  United States\\
  \texttt{\{ztyang,yilundu,lpk,tlp,jiayuanm\}@mit.edu}
}

\begin{document}
\maketitle

\input{text/6-supplementary}

\end{document}
